# Supplementary material for: Searching a Database of Source Codes Using Contextualized Code Search
Source: arXiv:2001.03277 source file (2020-07-26)
Supplement: Supplementary file 1 [file Appendix.tex]

\section{Appendix}
\subsection{Reverse Encoder in Multi Dimension}
\begin{equation*}
\begin{aligned}
P(Y|X) &= \int_Z P(Z|X)P(Y|Z) dZ \\
& = \int_Z \frac{P(Z|X)P(Z|Y)P(Y)}{P(Z)} dZ \\
& = \int_Z exp(A_1.Z^2 + B_1.Z + C_1.1) \times 
exp(A_2.Z^2 + B_2.Z + C_2.1) \\
& \times P(Y) \times exp(-A_I.Z^2 - B_I.Z- C_I.1) dZ
\end{aligned}
\end{equation*}

\begin{equation*}
\begin{aligned}
where &\\
&A_1 = <-\frac{1}{\sigma1_{ii}^2}>, B_1 = <\frac{\mu1_i}{\sigma1_{ii}^2}>, C_1 = < -\frac{\mu1_i^2}{2\sigma1_{ii}^2} - \frac{1}{2}ln2\pi - \frac{1}{2}ln(\sigma1_{ii}^2)>\\
&A_2 = <-\frac{1}{\sigma2_{ii}^2}>, B_2 = <\frac{\mu2_i}{\sigma2_{ii}^2}>, C_2 = < -\frac{\mu2_i^2}{2\sigma2_{ii}^2} - \frac{1}{2}ln2\pi - \frac{1}{2}ln(\sigma2_{ii}^2)> \\
& A_I = <-\frac{1}{2}> , B_I = <0>, C_I = <-\frac{1}{2}ln2\pi>
\end{aligned}
\end{equation*}

\begin{equation*}
\begin{aligned}
P(Y|X) &= P(Y) \int_Z exp(A_*.Z^2 + B_*.Z + C.1) dZ
&
\end{aligned}
\end{equation*}
where $A_* = A_1 + A_2 - A_I = <-\frac{1}{\sigma1_{ii}^2}-\frac{1}{\sigma2_{ii}^2} + \frac{1}{2}>$,\\
$B_* = B_1 + B_2 = <\frac{\mu1_i}{\sigma1_{ii}^2} + \frac{\mu2_i}{\sigma2_{ii}^2}>$,\\
$C = C_1+C_2-C_I = <-\frac{\mu1_i^2}{2\sigma1_{ii}^2} -
\frac{\mu2_i^2}{2\sigma2_{ii}^2} 
- \frac{1}{2}ln(\sigma1_{ii}^2)- \frac{1}{2}ln(\sigma2_{ii}^2) - \frac{1}{2}ln2\pi>$

\begin{equation*}
P(Y|X) = P(Y) \int_Z exp(A_*.Z^2 + B_*.Z + C_*.1) exp(C.1-C_*.1) dZ
\end{equation*}

$where \ \ C_* = <\frac{B_{*i}^2}{4A_{*i}} + \frac{1}{2}ln(-\frac{A_{*i}}{\pi})> $ \\
$ln P(Y|X) = ln P(Y) + \sum(C_i - C_{*i})$
\\
Also, 
\begin{equation*}
\begin{aligned}
C &= C_1 + C_2 - C_I \\
& = <\frac{B_{1i}^2}{4A_{1i}} + \frac{1}{2}ln(-\frac{A_{1i}}{\pi})> +  <\frac{B_{2i}^2}{4A_{2i}} + \frac{1}{2}ln(-\frac{A_{2i}}{\pi})> + <-\frac{1}{2} ln2\pi> \\
&= <\frac{B_{1i}^2}{4A_{1i}} + \frac{B_{2i}^2}{4A_{2i}} + \frac{1}{2}ln(-\frac{A_{1i}}{\pi})+  + \frac{1}{2}ln(-\frac{A_{2i}}{\pi}) + -\frac{1}{2} ln2\pi>
\end{aligned}
\end{equation*}

\begin{equation*}
\begin{aligned}
C - C_* & = 
&= <\frac{B_{1i}^2}{4A_{1i}} + \frac{B_{2i}^2}{4A_{2i}} - \frac{B_{*i}^2}{4A_{*i}} + \frac{1}{2}ln(-\frac{A_{1i}}{\pi}) + \frac{1}{2}ln(-\frac{A_{2i}}{\pi}) +
- \frac{1}{2}ln(-\frac{A_{*i}}{\pi}) -\frac{1}{2} ln2\pi>
\end{aligned}
\end{equation*}

\subsection{General Normal Form in Multi-Dimension}

\subsubsection{Prob of a point following a Normal Distribution if dim = 1}
$P(x|\mu,\sigma)  = \frac{1}{\sqrt{2\pi}\sigma}exp(-\frac{(x-\mu)^2}{2\sigma^2})$

\subsubsection{Prob of a point following a Normal Distribution if dim = d}

\begin{equation*}
\begin{aligned}
P(x|\mu,\sigma) &= \frac{1}{\sqrt{(2\pi)^d}\det(\Sigma)}exp(-\frac{1}{2}(x-\mu)^T\Sigma^{-1}(x-\mu)) \\
& = \frac{1}{(2\pi)^\frac{d}{2} (\prod_{1}^{d}\sigma_{ii}^2)^\frac{1}{2} }exp(-\frac{1}{2}\sum_{i=1}^{d}\frac{(x_i-\mu_i)^2}{\sigma_{ii}^2}) \\
ln P(x|\mu,\sigma) &= - \frac{1}{2}\sum_{1}^{d}\frac{(x_i-\mu_i)^2}{\sigma_{ii}^2} - \frac{d}{2} ln(2\pi) - \frac{1}{2}ln(\prod_{1}^{d} \sigma_{ii}^2) \\ 
  &= - \frac{1}{2}\sum_{1}^{d}\frac{(x_i-\mu_i)^2}{\sigma_{ii}^2} - \frac{d}{2} ln(2\pi) - \frac{1}{2}\sum_{1}^{d} ln( \sigma_{ii}^2) 
\end{aligned}
\end{equation*}

\subsubsection{Deriving 1-Dimensional Normal Form}

\begin{equation}
\begin{aligned}
P(x|\mu,\sigma)  &= \frac{1}{\sqrt{2\pi}\sigma}exp(-\frac{(x-\mu)^2}{2\sigma^2})\\
&=exp(ln(\frac{1}{\sqrt{2\pi}\sigma}))exp(-\frac{(x-\mu)^2}{2\sigma^2})\\
&=exp(ln(\frac{1}{\sqrt{2\pi}\sigma})-\frac{(x-\mu)^2}{2\sigma^2})
\end{aligned}
\end{equation}
Therefore, $ a=-\frac{1}{2\sigma^2}, b = \frac{\mu}{\sigma^2}, c = -\frac{1}{2}\frac{\mu^2}{\sigma^2} - \frac{1}{2}ln(2\pi)
- \frac{1}{2}ln(\sigma^2)$ \\
$where P(x|\mu,\sigma) = exp(ax^2 + bx + c)$ \\
$Also, \mu = -\frac{b}{2a}, \sigma^2 = -\frac{1}{2a}$ 
\\ and substituting in $c$ gives 
$c = \frac{b^2}{4a} + \frac{1}{2}ln(-\frac{a}{\pi})$

\subsubsection{Deriving the Normal Form in Multi-dimensions}
\begin{equation*}
\begin{aligned}
P(x|\mu,\sigma) &= \frac{1}{(2\pi)^\frac{d}{2}(\prod_{1}^{d}\sigma_{ii}^2)^\frac{1}{2}}exp(-\frac{1}{2}\sum_{i=1}^{d}\frac{(x_i-\mu_i)^2}{\sigma_{ii}^2}) \\
&= \frac{1}{(2\pi)^\frac{d}{2}(\prod_{1}^{d}\sigma_{ii}^2)^\frac{1}{2}}exp(\sum_{i=1}^{d} x_i^2\times(-\frac{1}{2\sigma_{ii}^2}) + \sum_{i=1}^{d} x_i \times(\frac{\mu_i}{\sigma_{ii}^2}) + \sum_{i=1}^{d}(-\frac{\mu_i^2}{2\sigma_{ii}^2} ) \\
&= \frac{1}{(2\pi)^\frac{d}{2}(\prod_{1}^{d}\sigma_{ii}^2)^\frac{1}{2}}exp(\sum_{i=1}^{d} x_i^2 \times a_i + \sum_{i=1}^{d} x_i \times b_i + \sum_{i=1}^{d} c_i^{'}) \\
\end{aligned}
\end{equation*}
\\
$where, \ \ a_i = -\frac{1}{2\sigma_{ii}^2}; \ b_i = \frac{\mu_i}{\sigma_{ii}^2};\  c_i^{'} = - \frac{\mu_i^2}{2\sigma_{ii}^2}$

\begin{equation*}
\begin{aligned}
P(x|\mu,\sigma) &= exp(-ln((2\pi)^\frac{d}{2}(\prod_{1}^{d}\sigma_{ii}^2)^\frac{1}{2}))exp(A.X^2 + B.X + C^{'}.1) \\
&=exp(-\frac{d}{2}ln(2\pi) - \frac{1}{2}\sum_{1}^{d}ln(\sigma_{ii}^2)) 
\times exp(AX^2 + BX + C^{'}.1) \\
&=exp(AX^2 + BX + \sum_{1}^{d}(- \frac{\mu_i^2}{2\sigma_{ii}^2} - \frac{1}{2}ln2\pi - \frac{1}{2} ln(\sigma_{ii}^2)) )\\
&=exp(AX^2 + BX + C.1)
\end{aligned}
\end{equation*}
$where, \ \ A = <-\frac{1}{2\sigma_{ii}^2}>; \ B = <\frac{\mu_i}{\sigma_{ii}^2}> ;\ C = <- \frac{\mu_i^2}{2\sigma_{ii}^2} -\frac{1}{2}ln(2\pi) - \frac{1}{2}ln(\sigma_{ii}^2)>$\
Note that the scalars add up over $d$ dimensions.\\

\subsubsection{Deriving relations between A, B and C}

$A = <-\frac{1}{2\sigma_{ii}^2}>$
$B = <-\frac{\mu_i}{2\sigma_{ii}^2}>$
$C = <-\frac{\mu_i^2}{2\sigma_{ii}^2} - \frac{1}{2}ln2\pi - \frac{1}{2}ln(\sigma_{ii}^2)>$ $i=1..d$
\\
$A_i = -\frac{1}{2\sigma_{ii}^2}$
$B_i = -\frac{\mu_i}{2\sigma_{ii}^2}$
$C_i = -\frac{\mu_i^2}{2\sigma_{ii}^2} - \frac{1}{2}ln2\pi - \frac{1}{2}ln(\sigma_{ii}^2)$
\\
$\sigma_{ii}^2 = -\frac{1}{2A_i}$
$\mu_{i} = -\frac{B_i}{2A_i}$
\\
Substituting $\sigma$ and $\mu$ values in $C_i$ \\
$C_i = -\frac{\frac{B_i^2}{4A_i^2}}{2\frac{-1}{2A_i}}  - \frac{1}{2}ln(\frac{-1}{2A_i}) - \frac{1}{2}ln2\pi$ \\
$=\frac{B_i^2}{4A_i} - \frac{1}{2}ln(-\frac{1}{2A_i}) - \frac{1}{2}ln(2\pi)$
$=\frac{B_i^2}{4A_i} - \frac{1}{2}ln(-\frac{\pi}{A_i})$
$=\frac{B_i^2}{4A_i} + \frac{1}{2}ln(-\frac{A_i}{\pi})$ \\

\subsection{KL Divergence}
\subsection{KL between two Multi-variate Gaussians}
$D_{KL}(\mathcal{N}(\mu_1, \Sigma_1) \parallel \mathcal{N}(\mu_2, \Sigma_2)) = \\ \frac{1}{2} [ log\frac{\det \Sigma_2}{\det \Sigma_1} -d + tr\{\Sigma_2^{-1} \Sigma_1\} + (\mu_2 - \mu_1)^T\Sigma_2^{-1}(\mu_2 - \mu_1) ] $ \\
\\
Assuming $\Sigma_1$ and $\Sigma_2$ are diagonal matrices
\\
\begin{equation*}
\begin{aligned}
log \frac{\det \Sigma_2}{\det \Sigma_1} &= log \frac{\prod_{i}\Sigma_2^{ii}}{\prod_{i}\Sigma_1^{ii}} \\
&=log {\prod_{i}\Sigma_2^{ii}} - log {\prod_{i}\Sigma_1^{ii}}\\
&= \sum_{i}log\Sigma_2^{ii} - \sum_{i}log\Sigma_1^{ii} \\
&= \sum_{i}log (\sigma_2^{ii})^2 - \sum_{i}log(\sigma_1^{ii})^2
\end{aligned}
\end{equation*} \\

$tr\{\Sigma_2^{-1} \Sigma_1\} = \sum_{i=1}^{d}\frac{(\sigma_1^{ii})^2}{(\sigma_2^{ii})^2}$\\
$(\mu_2 - \mu_1)^T\Sigma_2^{-1}(\mu_2 - \mu_1) = \sum_{i=1}^{d} \frac{(\mu_2 - \mu_1)^2}{(\sigma_2^{ii})^2}$ \\

$D_{KL}(\mathcal{N}(\mu_1, \Sigma_1) \parallel \mathcal{N}(\mu_2, \Sigma_2)) = \\ \frac{1}{2} [ \sum_{i}log (\sigma_2^{ii})^2 - \sum_{i}log(\sigma_1^{ii})^2 -d + \sum_{i=1}^{d}\frac{(\sigma_1^{ii})^2}{(\sigma_2^{ii})^2} + \sum_{i=1}^{d} \frac{(\mu_2 - \mu_1)^2}{(\sigma_2^{ii})^2} ]$ \\

\subsection{Alternate Derivation to train our Search 
Model}
\begin{equation*}
\begin{aligned}
KL(Q(Z|Y) || P(Z|XY)) &= E_{Z \sim q_{\psi}}(Z|Y)[log_Q(Z|Y) - log_P(Z|XY)] \\
&=E_{Z \sim Q(Z|Y)}[log_Q(Z|Y) - log_P(YZ|X) + log_P(Y|X)]\\
\end{aligned} 
\end{equation*}

\begin{equation*}
\begin{aligned}
&E_{Z \sim Q(Z|Y)}[log Q(Z|Y) - log P(YZ|X) + log P(Y|X)] >= 0 \\
&log P(Y|X) >= E_{Z \sim Q(Z|Y)}[- log Q(Z|Y) + log P(YZ|X)] \\
&log P(Y|X) >= E_{Z \sim Q(Z|Y)}[- log Q(Z|Y) + log P(Y|ZX) + log P(Z|X) ] \\
&log P(Y|X) >= -KL(q_{\psi(Z|Y)} || P(Z|X)) + E_{Z \sim Q(Z|Y)}[ log P(Y|Z) ] \\
\end{aligned} 
\end{equation*}
